# Supplementary material for: Local SGD for Near-Quadratic Problems: Improving Convergence under Unconstrained Noise Conditions
Source: arXiv:2409.10478 source file (2024-12-18)
Supplement: Supplementary file 1 [file VeryEnd.tex]

\begin{lemma} \label{lem:decay_eps}
    Suppose $F$ is convex and has Lipschitz Hessian, meaning that $F$ is twice differentiable and exists such constant $\frac{C}{6}$, that for any $x, y \in \mathbb{R}$:
    \begin{align}
        \norm{\nabla^2 F(x) - \nabla^2 F(y)} \leq \frac{C}{6} \norm{x-y}
    \end{align}

    Also let us define $L^{\mathbb{S}}$-smoothness as regular $L$-smoothness on some subset $\mathbb{S} \subset \mathbb{R}^d$.

    Then, for some distributed algorithm $\mathcal{A}$ involving $M$ devices with corresponding local weights $x^m_t$ it holds that $L^{\mathbb{S}_t}_R \leq 2C \cdot \text{max} \{ \norm{x^m_t - x_*} \}$ for all sets $\mathbb{S}_t \in \mathbb{R}^d$ containing all of $x^m_t$.

    \begin{proof}
    \cite{Nesterov} in his Lemma 1.2.4 proved that if $F$ satisfies Lipschitz Hessian assumption, then for all $x, y \in \mathbb{R}$

    \begin{align}
         \norm{\nabla F(x) - \nabla F(y) - \nabla^2 F(x)(y-x)} \leq \frac{C}{2} \norm{x-y}^2 \label{eq:2404_4}
    \end{align}    
    
    Statement~\ref{st:st_1} holds for any decompositions of $F$ as the sum of $Q$ and $R$. Thus, we are free to choose $Q$ and $R$ in way that minimizes $\frac{L_R}{L}$ on each step. Thus, let us naturally define

    R невыпуклая

    \begin{align}
        &Q(x) := F(x_*) + \inner{\nabla F(x_*)}{x-x_*} + \frac{1}{2} \inner{\nabla^2 F(x_*)(x-x_*)}{x-x_*} \\
        &= F(x_*) + \frac{1}{2} \inner{\nabla^2 F(x_*)(x-x_*)}{x-x_*} \\
        &R(x) := F(x) - Q(x)
    \end{align}

    So, $F(x) = Q(x) + R(x)$ and $Q$ is quadratic.

    \vspace{10pt}

    Denoting $H = \nabla^2 F(x_*)$ following facts can be shown:

    \begin{align}
        &Q(x) = F(x_*) + (x-x_*)^T H (x-x_*) \\
        &\nabla Q(x) = H (x-x_*) \\
        &\nabla^2 Q(x) = H
    \end{align}

    Thus,
    \begin{align}
        &\nabla Q(x_*) = 0 \\
        &\nabla^2 Q(x_*) = \nabla^2 F(x_*) \\
        &\nabla R(x_*) = F(x_*) - Q(x_*) = 0 \\
        &\nabla^2 R(x_*) = \nabla^2 F(x_*) - \nabla^2 Q(x_*) = 0
    \end{align}

    Substituting this into \eqref{eq:2404_4} we gain:
    \begin{align}
        &\norm{\nabla R(x) + \nabla Q(x) - \nabla R(x_*) - \nabla Q(x_*) - \nabla^2 Q(x_*)(x-x_*) - \nabla^2 R(x_*) (x-x_*)} \\
        &=
        \norm{\nabla R(x) + H(x-x_*) - H(x-x_*)}
        =
        \norm{\nabla R(x)}
        \leq \frac{C}{2} \norm{x-x_*}^2
    \end{align}

    Thus, for any such $y$ that $\norm{y-x_*} \leq \norm{x-x_*}$,

    \begin{align}
        \norm{\nabla R(x) - \nabla R(y)} \leq C \norm{x-x_*} \cdot \norm{x-y}.
    \end{align}

    Which proves the claimed fact.
    \end{proof}
\end{lemma}
